# Supplementary material for: HPO-B: A Large-Scale Reproducible Benchmark for Black-Box HPO based on OpenML
Source: arXiv:2106.06257 source file (2021-10-11)
Supplement: Supplementary file 1 [file supplementary-bench.tex]

\documentclass{article}

\begin{document}

\end{document}
